# Supplementary material for: On Predicting Generalization using GANs
Source: arXiv:2111.14212 source file (2022-03-17)
Supplement: Supplementary file 1 [file appendix.tex]

\section{Appendix}

\subsection{Conditional Mutual Information} 
\citet{jiang2019fantastic} Let $\Theta$ be the hyper-parameter space, $\Theta_i$ an axis of that space (i.e. a particular hyper-parameter), $g(\theta), \theta \in \Theta$ be the generalization gap given some hyper-parameter configuration and $\mu(\theta), \theta \in \tau$ the complexity measure. Let $\mathcal{S}$ be a hyper-parameter type, e.g. learning rate. Let $\mathcal{U}_{\mathcal{S}}$ be a random variable corresponding to the values of the hyper-parameters in $\mathcal{S}$. Let $\phi : \Theta \rightarrow \mathbb{R}$ be any function, $V_{\phi} : \Theta_i \times \Theta_2 \rightarrow {-1, +1}$ be defined as $V_{\phi}(\theta_1, \theta_2) = sign(\phi(\theta_1) - \phi(\theta_2)) $. The conditional mutual information is defined as follows:
\begin{equation}
    \mathcal{I}(V_{\mu}, V_{g} \vert \mathcal{U}_s) = \sum_{\mathcal{U}_\mathcal{S}} p(\mathcal{U}_{\mathcal{S}}) \sum_{V_{\mu}\in {\{\pm 1\}}} \sum_{V_{g}\in \{\pm 1\}} p(V_{\mu}, V_g \vert \mathcal{U}_{\mathcal{S}}) \log \left( \frac{p(V_\mu ,V_g \vert \mathcal{U}_{\mathcal{S}})}{p(V_{\mu} \vert \mathcal{S}) p(V_g \vert \mathcal{U}_\mathcal{S})} \right)
\end{equation}
